# Supplementary material for: DeepSport: A Multimodal Large Language Model for Comprehensive Sports Video Reasoning via Agentic Reinforcement Learning
Source: arXiv:2511.12908 source file (2026-03-11)
Supplement: Supplementary file 1 [file X_suppl.tex]

\clearpage
\setcounter{page}{1}
\maketitlesupplementary

\section{Prompt}

\begin{tcolorbox}[mybox, breakable]
{\small\ttfamily
You are an expert AI assistant that answers questions about
a video by iteratively analyzing it.

\vspace{0.5em}
\# Tools

\vspace{0.5em}
You can call the tool defined below to **uniformly sample
frames** within a given frame index range.

\vspace{0.5em}
\textless tools\textgreater\\
{[}\\
\hspace*{1em}\{\\
\hspace*{2em}``type'': ``function'',\\
\hspace*{2em}``function'': \{\\
\hspace*{3em}``name'': ``choose\_frames'',\\
\hspace*{3em}``description'': ``Uniformly sample frames within the provided frame index range. If there are specific moments you want to inspect, invoke this tool to fetch the corresponding frames. In typical usage, you first receive 8 preview frames; you can then pick two frame indices from those previews and call this tool again with {[}start, end{]} to uniformly re-sample frames between them for closer, fine-grained observation.'',\\
\hspace*{3em}``parameters'': \{\\
\hspace*{4em}``type'': ``object'',\\
\hspace*{4em}``properties'': \{\\
\hspace*{5em}``frame\_range'': \{\\
\hspace*{6em}``type'': ``array'',\\
\hspace*{6em}``items'': \{ ``type'': ``integer'' \},\\
\hspace*{6em}``minItems'': 2,\\
\hspace*{6em}``maxItems'': 2,\\
\hspace*{6em}``description'': ``{[}START\_FRAME, END\_FRAME{]} as frame indices.''\\
\hspace*{5em}\}\\
\hspace*{4em}\},\\
\hspace*{4em}``required'': {[}``frame\_range''{]}\\
\hspace*{3em}\}\\
\hspace*{2em}\}\\
\hspace*{1em}\}\\
{]}\\
\textless /tools\textgreater

\vspace{0.5em}
\# How to call the tool (**strict** json format)

\vspace{0.5em}
Return **exactly one** tool call JSON wrapped in
`\textless tool\_call\textgreater' tags. If no sampling is
needed, answer the question directly in text without any
tool call or extra wrapper text.

\vspace{0.5em}
\# Example (your single call should look exactly like this)

\vspace{0.5em}
\textless tool\_call\textgreater\{\\
``action'': ``choose\_frames'',\\
``frame\_range'': {[}START\_FRAME, END\_FRAME{]}\\
\}\textless /tool\_call\textgreater

\vspace{0.5em}
Start you output with \textless think\textgreater. You need
to analyze the frames within a
\textless think\textgreater\textless /think\textgreater\ tag.
After thinking with the frames, choose one of the following:

\vspace{0.5em}
1. If you are not sure about the answer, you can continue\\
\hspace*{1.5em}with:\\
\textless tool\_call\textgreater\{\\
\hspace*{1em}``action'': ``choose\_frames'',\\
\hspace*{1em}``frame\_range'': {[}START\_FRAME, END\_FRAME{]}\\
\}\textless /tool\_call\textgreater\\
\hspace*{1.5em}to gain more frames.

\vspace{0.5em}
2. If you are positive with your final answer, you can\\
\hspace*{1.5em}provide the final answer within a\\
\hspace*{1.5em}\textless answer\textgreater\textless /answer\textgreater\
~tag.

\vspace{0.5em}
All your thinking processes should be a concise, logical,
visual-based chain-of-thought. Think naturally as a human
would, using inner dialogue like ``let me think,'' ``hmm,''
``wait,'' etc.
}
\end{tcolorbox}
\captionof{figure}{System Prompt for DeepSport: The agent is instructed to iteratively analyze video frames using the \texttt{choose\_frames} tool.}

\begin{tcolorbox}[mybox, breakable]
{\small\ttfamily
\{\$Question\}

\vspace{0.5em}
frame \{\$FrameIdx\_1\}: \textless image\textgreater\\
frame \{\$FrameIdx\_2\}: \textless image\textgreater\\
frame \{\$FrameIdx\_3\}: \textless image\textgreater\\
...\\
frame \{\$FrameIdx\_N\}: \textless image\textgreater
}
\end{tcolorbox}
\captionof{figure}{User Prompt for DeepSport: \texttt{\$Question} is replaced with the actual question text, and \texttt{\$FrameIdx\_*} are replaced with uniformly sampled frame indices from the video.}

\begin{tcolorbox}[mybox, breakable]
{\small\ttfamily
You are a scoring assistant for sports questions.

\vspace{0.5em}
Rules

\vspace{0.5em}
Compare the semantic meaning of ``ground truth'' and ``model response'' and assign a similarity score between 0 (completely different) and 1 (meaning identical).

\vspace{0.5em}
Output

\vspace{0.5em}
Return ONLY one line: (replace the score to the real number)

\vspace{0.5em}
\textless answer\textgreater score\textless /answer\textgreater

\vspace{0.5em}
Now is your turn

\vspace{0.5em}
- question: \{\$Question\}\\
- sport: \{\$SPORT\}\\
- ground truth: \{\$Truth\}\\
- model response: \{\$ModelAnswer\}
}
\end{tcolorbox}
\captionof{figure}{RL Reward Prompt: \texttt{\$Question}, \texttt{\$SPORT}, \texttt{\$Truth}, and \texttt{\$ModelAnswer} are replaced with actual sample fields.}

\begin{tcolorbox}[mybox, breakable]
{\small\ttfamily
You are responsible for proofreading the answers, you need to give a score to the model's answer by referring to the standard answer, based on the given question. The full score is 1 point and the minimum score is 0 points. Please output the score in the json form ``\{score: \textless score\textgreater\}''. The evaluation criteria require that the closer the model's answer is to the standard answer, the higher the score.

\vspace{0.5em}
Question: \{\$Question\}

\vspace{0.5em}
Standard answer: \{\$Standard\_answer\}

\vspace{0.5em}
Model's answer: \{\$Model\_answer\}

\vspace{0.5em}
Sport: \{\$Sport\}
}
\end{tcolorbox}
\captionof{figure}{Evaluation Prompt: \texttt{\$Question}, \texttt{\$Standard\_answer}, \texttt{\$Model\_answer}, and \texttt{\$Sport} are replaced with actual sample fields.}

\section{Experiment Details}
\subsection{Traning Details}
Figure~\ref{tool_call_mean} and Figure~\ref{reward_mean} illustrate the training dynamics of our GRPO framework over 300 steps. The tool call mean (Figure~\ref{tool_call_mean}) measures the frequency of frame sampling tool invocations by the agent. The curve demonstrates a rapid increase from 0.3 to 0.8 within the first 100 steps, subsequently converging to approximately 0.9. This indicates that the agent learns to actively utilize the iterative frame sampling mechanism for video analysis.

The reward curve (Figure~\ref{reward_mean}) shows the evaluation scores assigned by the critic model. The mean reward improves from 0.3 to 0.55 over the training period, with the smoothed trajectory exhibiting consistent upward trends. The correlation between increased tool usage and improved reward validates that iterative visual reasoning contributes to more accurate question answering on the DeepSport benchmark.

\begin{figure}
    \centering
    \includegraphics[width=0.95\linewidth]{author-kit-CVPR2026-v1-latex-//sec//appendix/tool\_call\_curve.png}
    \caption{Tool Call Mean Curve}
        \label{tool_call_mean}
\end{figure}

\begin{figure}
        \centering
        \includegraphics[width=0.95\linewidth]{author-kit-CVPR2026-v1-latex-//sec//appendix/reward\_curve.png}
        \caption{Reward Mean Curve}
        \label{reward_mean}
\end{figure}
\subsection{Reward Function Details}

\begin{table*}[t]
\centering
\caption{Ablation on the effect of training stages.}
\label{tab:model_abl}
\resizebox{0.97\textwidth}{!}{%
\large

\begin{tabular}{l|c|cccc|c}
\toprule
\textbf{Model} & \textbf{Frames} & \textbf{Fine-Grained} & \textbf{Rule \&} & \textbf{Assessment \&} & \textbf{Live Commentary} & \textbf{Overall} \\
& & \textbf{Recognition} & \textbf{Procedural} & \textbf{Coaching} & \textbf{\& Reporting} & \textbf{Avg.} \\
\midrule
Qwen2.5-VL-7B-Instruct & 16 & 28.20 & 13.71 & 9.09 & 3.13 & 16.98 \\
Qwen2.5-VL-7B-Instruct (SFT) & \textbf{10} & 40.67 & 24.38 & 21.40 & 21.07 & 29.91 \\
\midrule
\textbf{DeepSport} & 14.39 & \textbf{51.09} & \textbf{43.82} & \textbf{24.74} & \textbf{24.60} & \textbf{40.08} \\
\bottomrule
\end{tabular}%
}
\end{table*}

We provide implementation details for the Gated Tool-Use Reward Function introduced in Section~\ref{par:reward}.

\noindent\textbf{Format Validation ($g_{\text{fmt}}$).}
The format gate $g_{\text{fmt}}(\tau)$ enforces structural integrity through the following validation rules:

\textit{Tag Matching.} We verify that:
\begin{itemize}
    \item the number of \texttt{<think>} equals \texttt{</think>},
    \item the number of \texttt{<tool\_call>} equals \texttt{</tool\_call>},
    \item exactly one pair of \texttt{<answer>} and \texttt{</answer>} exists, and
    \item $\#\{\texttt{<think>}\} = \#\{\texttt{<tool\_call>}\} + 1$.
\end{itemize}

\textit{Nesting Rules.} Content within \texttt{<think>...</think>} and \texttt{<answer>...</answer>} must not contain other tags. All tag pairs must have non-empty content.

\textit{Tool Call Validation.} Each \texttt{<tool\_call>} must contain valid JSON with format \texttt{\{"action": "choose\_frames", "frame\_range": [start, end]\}}. We enforce $\text{start} \le \text{end} - 8$ (minimum 8 frames) and prohibit redundant exploration: the new start index cannot equal the previous interval's endpoints.

\noindent\textbf{Accuracy Scoring ($\text{acc}(\tau)$).}
We employ LLM-as-Judge using DeepSeek-V3.2-Exp~\cite{deepseekai2024deepseekv32} to evaluate semantic similarity between the model's answer and ground truth. The judge is prompted to assign a score in $[0,1]$ based on semantic equivalence, not surface-level string matching. Invalid responses default to 0.0.

\section{Ablation Study}
\begin{figure*}[htp]
    \centering
    \includegraphics[width=0.97\textwidth]{author-kit-CVPR2026-v1-latex-//sec//appendix/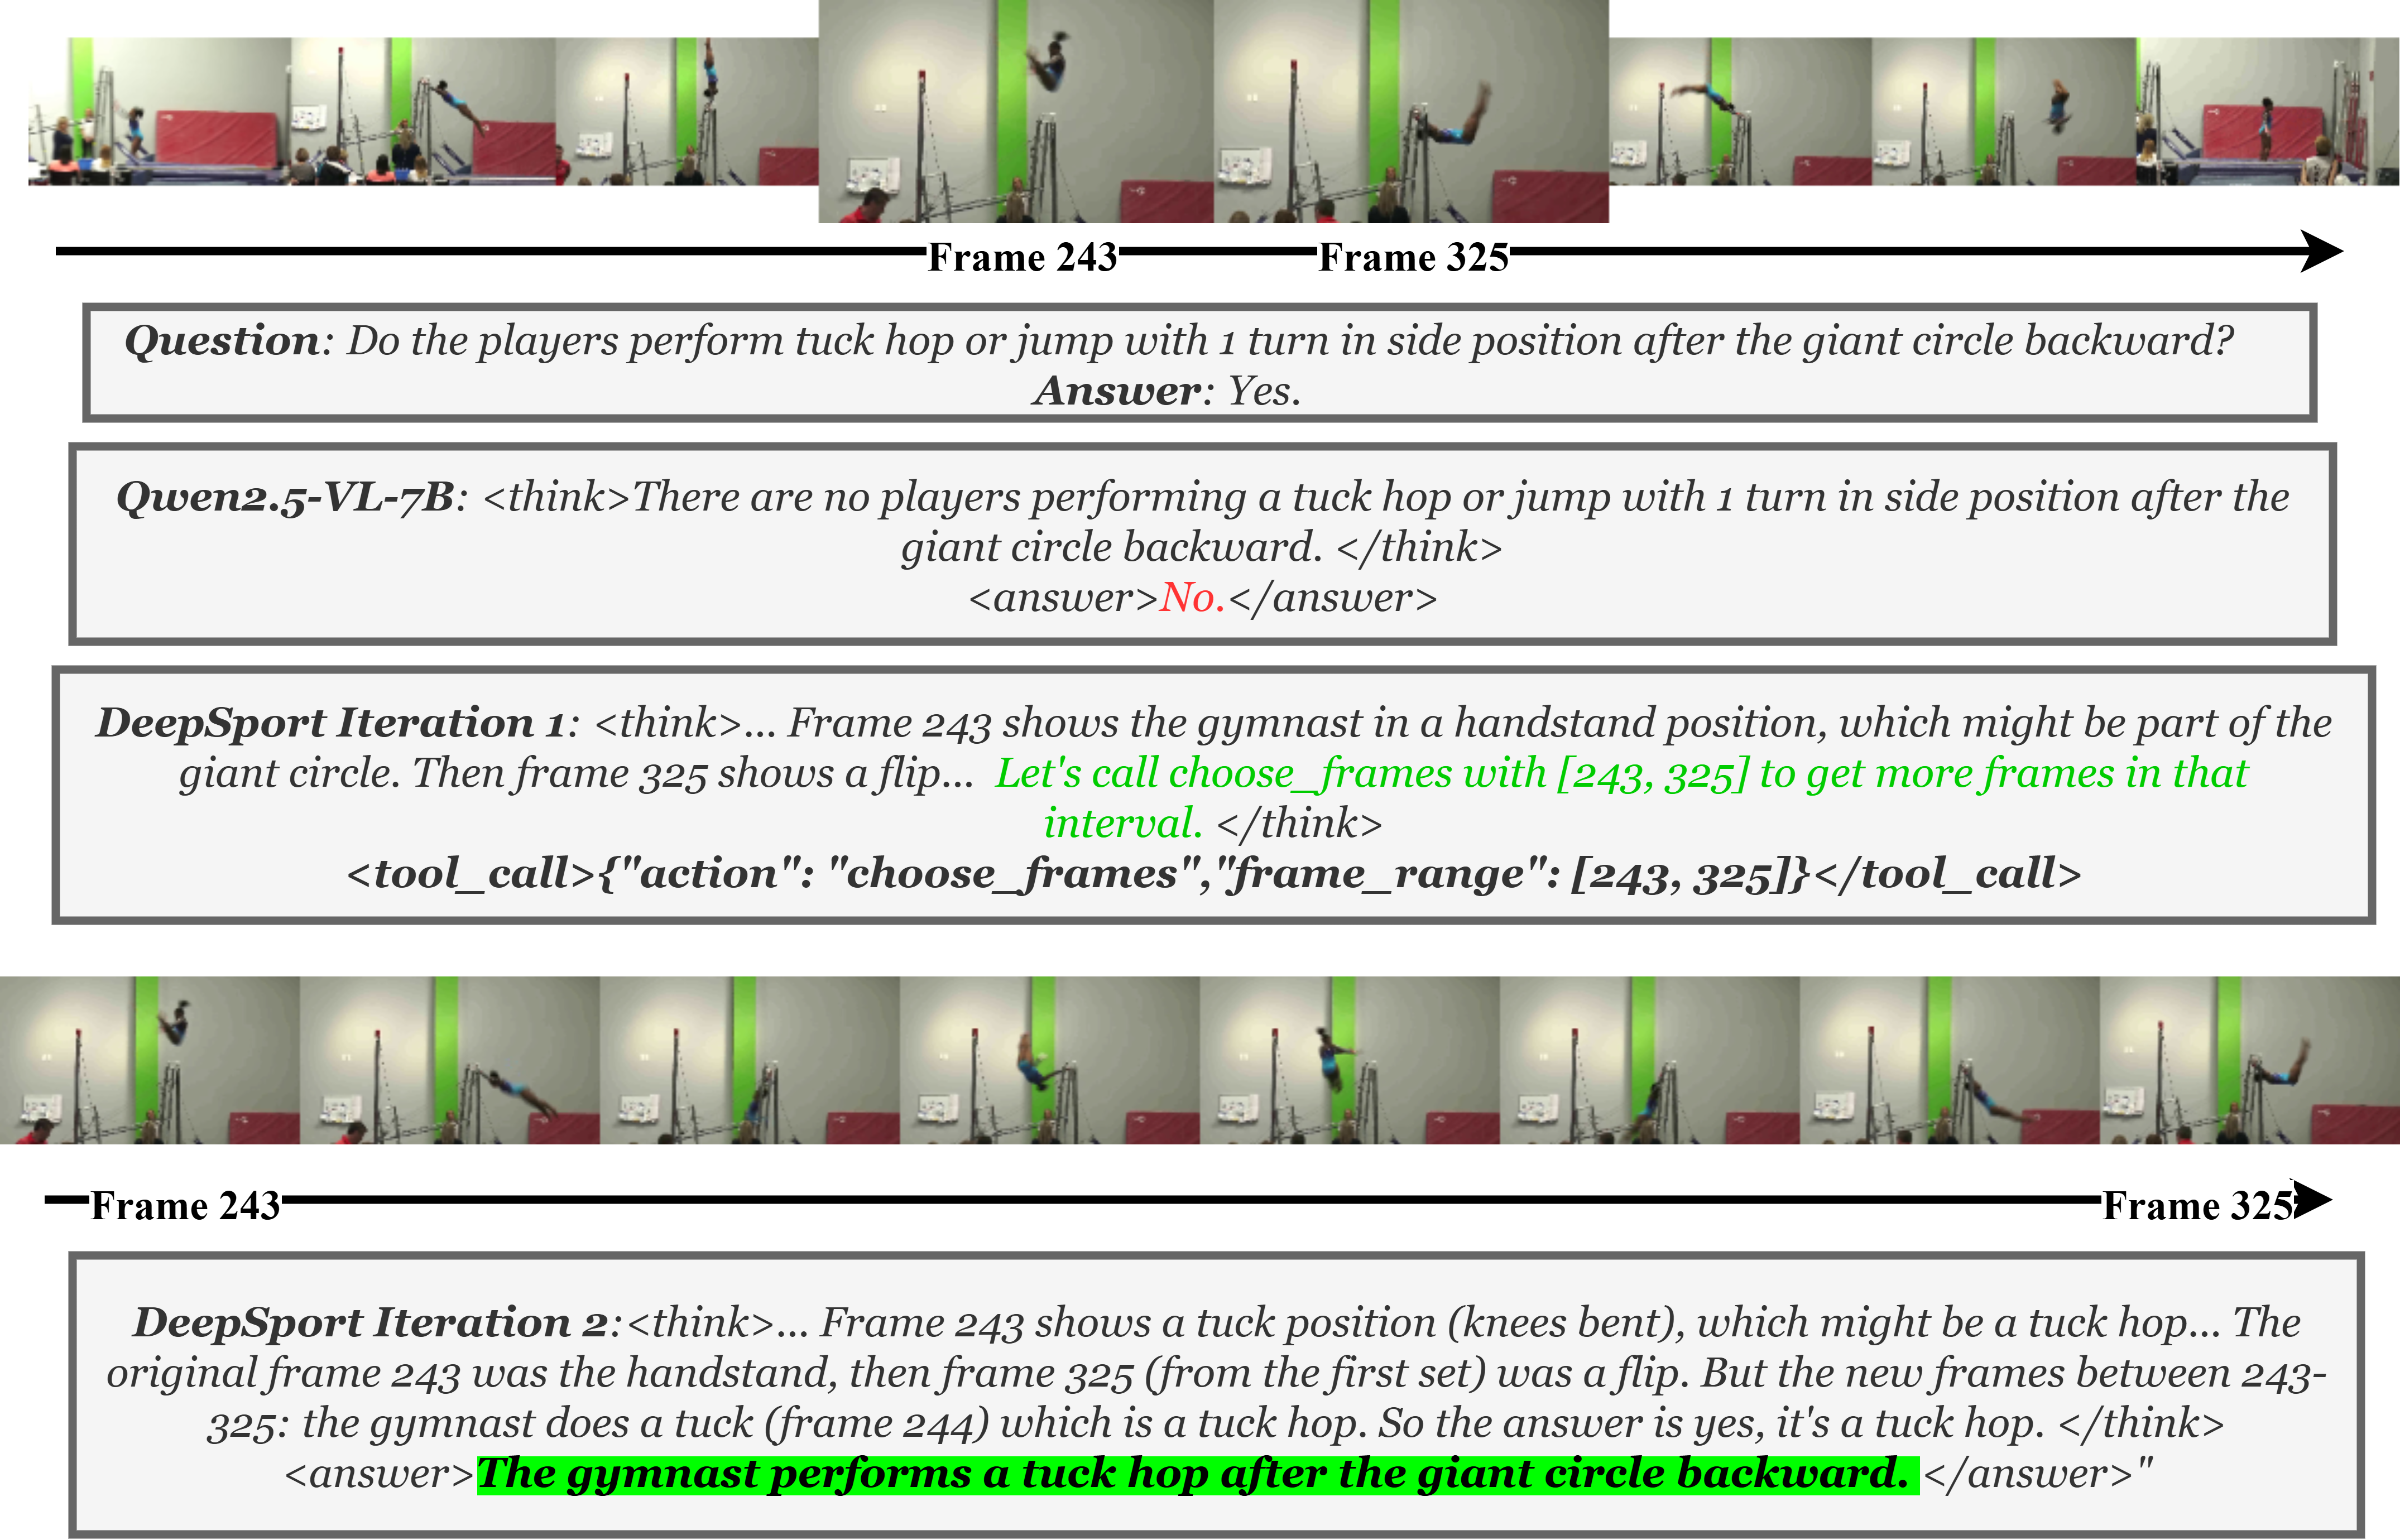}
    \caption{DeepSport Sample 1}
    \label{case1}
\end{figure*}
Table~\ref{tab:model_abl} demonstrates the effectiveness of our two-stage training pipeline. The baseline Qwen2.5-VL-7B-Instruct model, which uniformly samples 16 frames without tool-based frame extraction, achieves 16.98\% overall accuracy. After SFT on the DeepSport-CoT-15k dataset, the model learns the basic tool-calling syntax and iterative reasoning patterns, resulting in a substantial improvement to 29.91\% (+12.93 points) while reducing average frame usage to 10 frames. This validates that SFT successfully teaches the model \textit{how} to invoke tools and structure multi-turn trajectories.

However, SFT alone is insufficient for optimal tool utilization and video understanding. Our full DeepSport model, trained with GRPO-based agentic reinforcement learning, achieves 40.08\% overall accuracy (+10.17 points over SFT), with particularly notable gains in Fine-Grained Recognition (+10.42) and Rule \& Procedural tasks (+19.44). The RL phase refines the model's exploration strategy, as evidenced by the increased average frame usage (14.39 frames), indicating more adaptive and thorough video analysis. This ablation confirms that while SFT provides essential cold-start capabilities, reinforcement learning is critical for developing sophisticated tool-use policies and deeper video comprehension.

\section{Case Study}
Figure~\ref{case1} and Figure~\ref{case2} show examples from our dataset. We also plan to release our dataset later.

\section{Error Analysis}
Figures~\ref {errorincomplete} to~\ref {errordomain} show detailed error examples. Also, our model has already surpassed the average score of other SOTA models; however, our model still shows errors. Future work should focus on how to address these errors to achieve a stronger model.

\begin{figure*}[htp]
    \centering
    \includegraphics[width=0.97\textwidth]{author-kit-CVPR2026-v1-latex-//sec//appendix/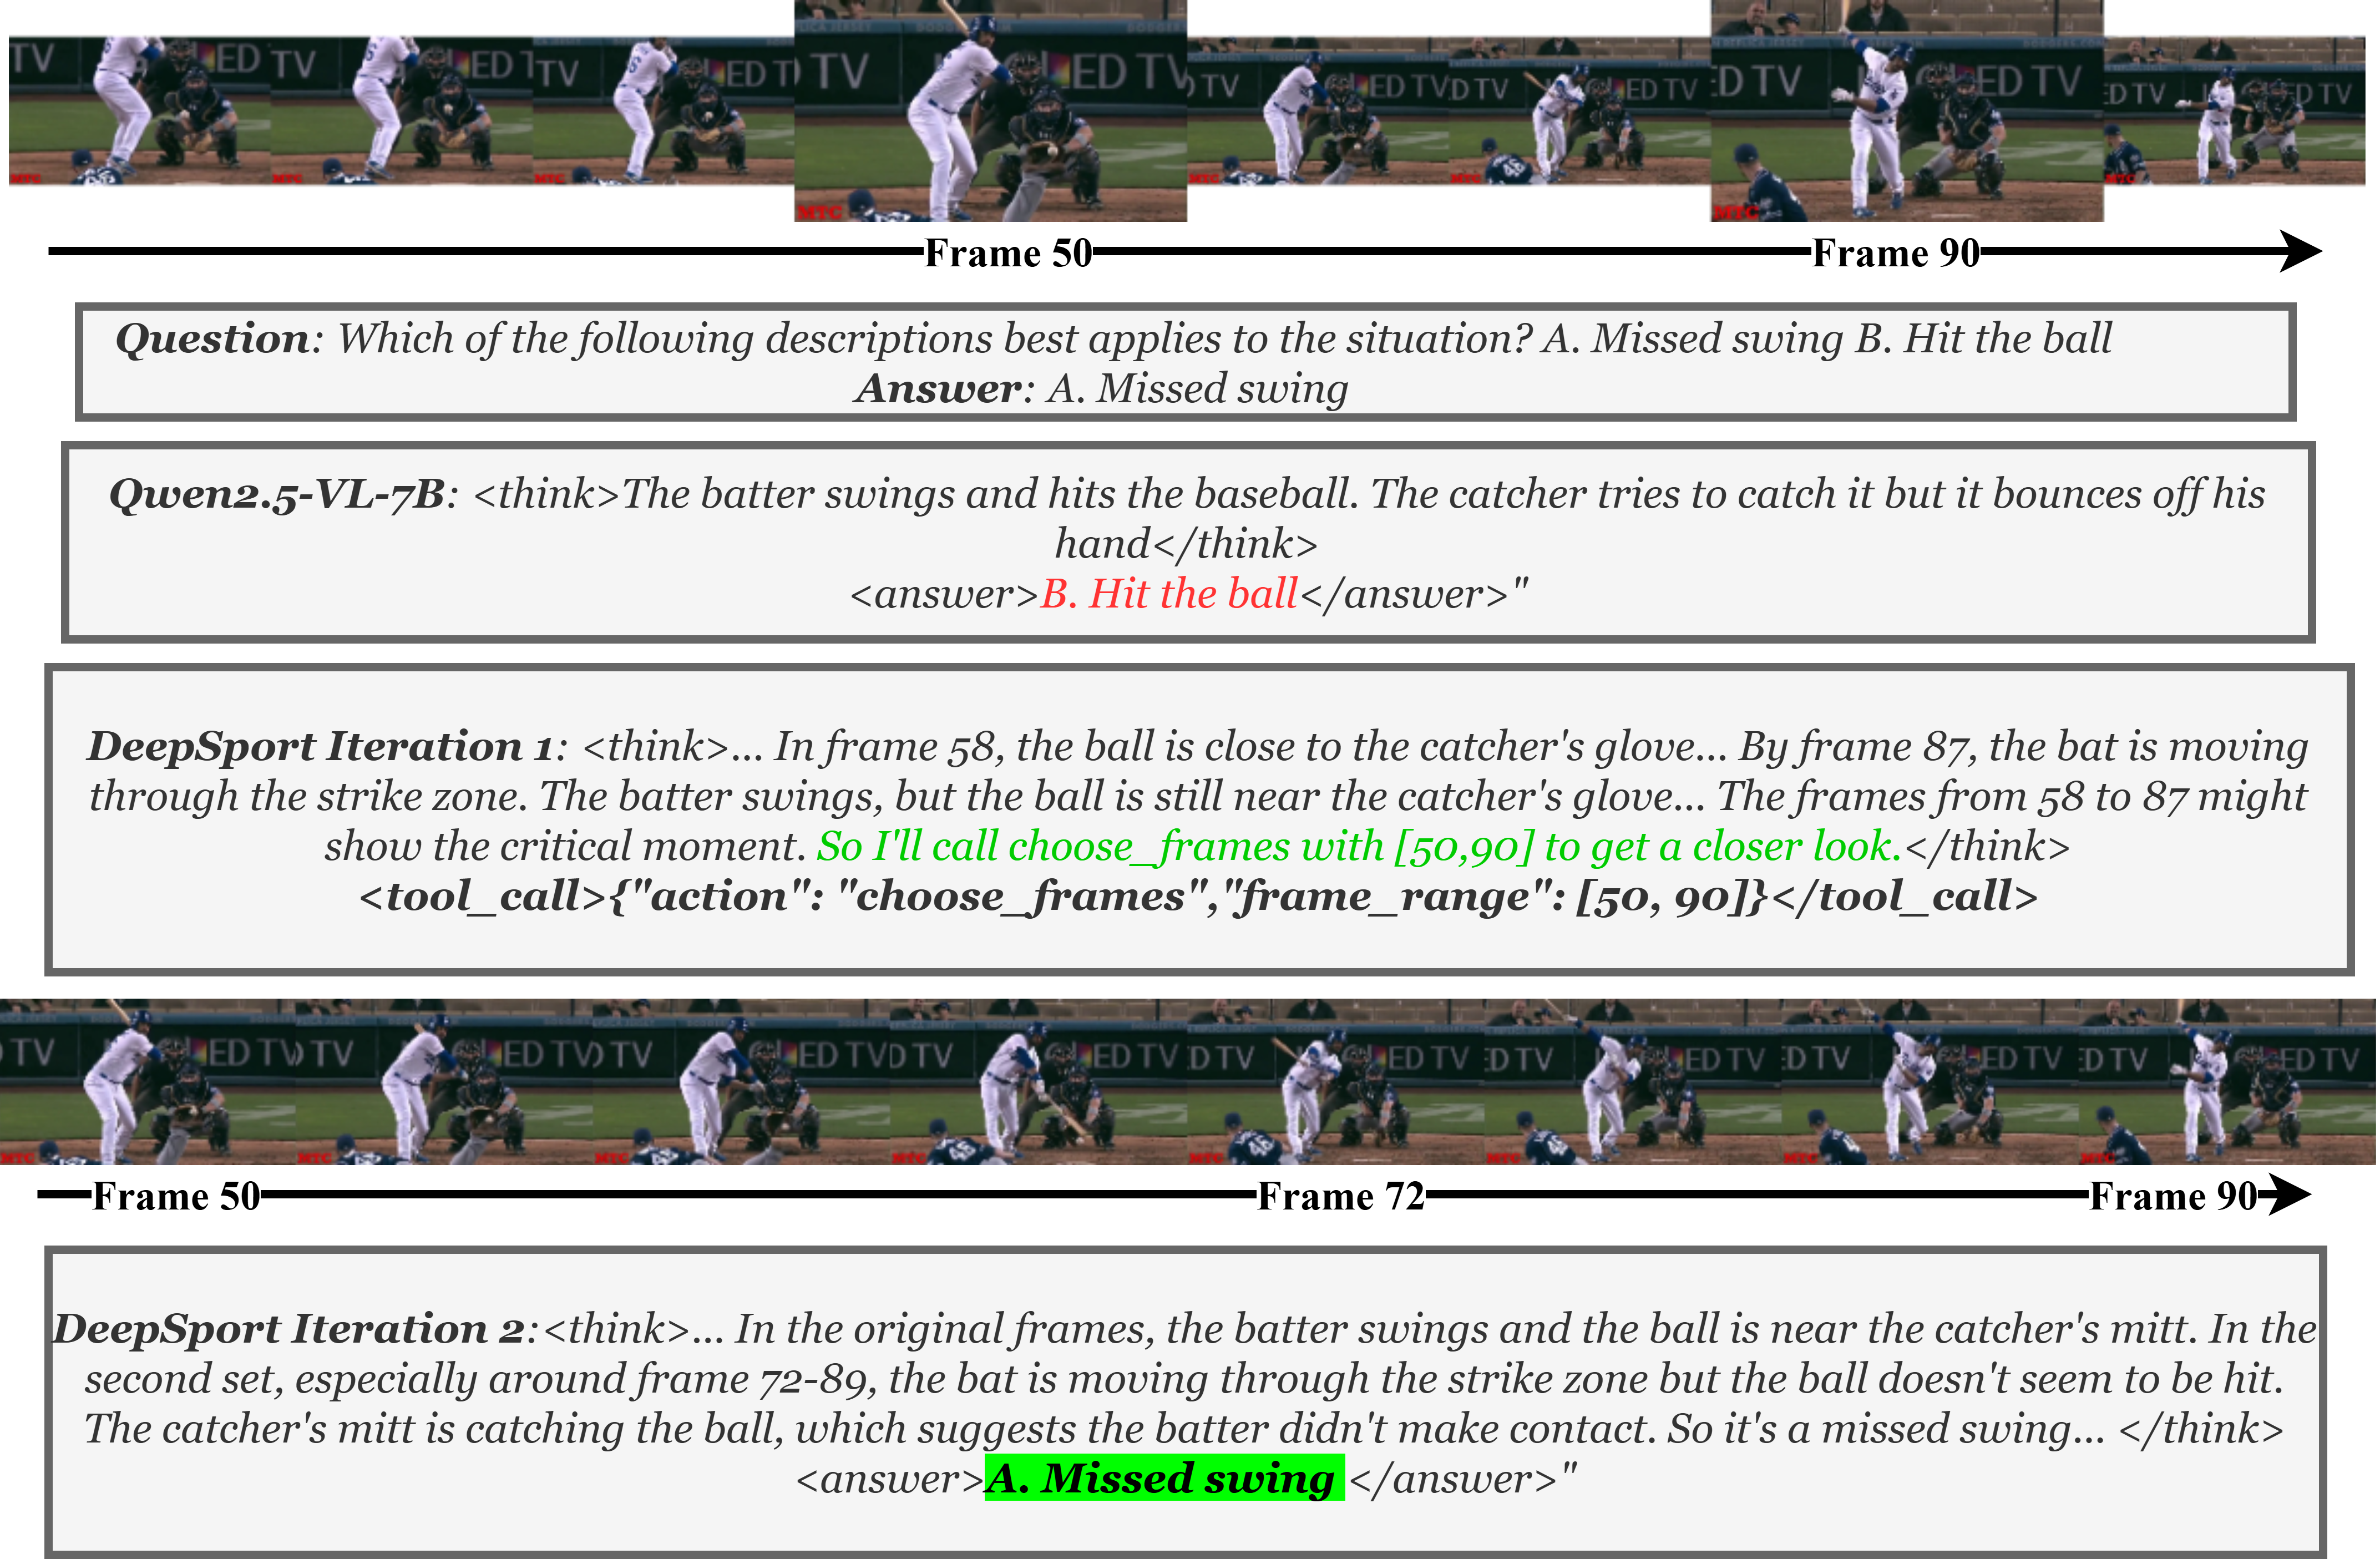}
    \caption{DeepSport Sample 2}
    \label{case2}
\end{figure*}

\begin{figure*}[htp]
    \centering
    \includegraphics[width=0.70\textwidth]{author-kit-CVPR2026-v1-latex-//sec//appendix/error2}
    \caption{Incomplete Exploration Example}
    \label{errorincomplete}
\end{figure*}

\begin{figure*}[htp]
    \centering
    \includegraphics[width=0.70\textwidth]{author-kit-CVPR2026-v1-latex-//sec//appendix/error3}
    \caption{Tool Failure Example}
    \label{errortool}
\end{figure*}

\begin{figure*}[htp]
    \centering
    \includegraphics[width=0.70\textwidth]{author-kit-CVPR2026-v1-latex-//sec//appendix/error4}
    \caption{Visual Hallucination Example}
    \label{errorvisual}
\end{figure*}

\begin{figure*}[htp]
    \centering
    \includegraphics[width=0.70\textwidth]{author-kit-CVPR2026-v1-latex-//sec//appendix/error5}
    \caption{Domain Knowledge Gap Example}
    \label{errordomain}
\end{figure*}
